# Supplementary material for: SQLCheck: Automated Detection and Diagnosis of SQL Anti-Patterns
Source: arXiv:2004.10232 source file (2020-04-21)
Supplement: Supplementary file 1 [file additional-experiments.tex]

\newcommand{\nexp}{15}
% \subsection{Additional Applications:}
We tested \sys on \nexp  open-source database applications which use an ORM. For this experiment, we integrated \sys with the test pipeline of these applications, where the queries executed during the integration tests are analyzed by \sys for detecting \apsshort. We adjusted the ranking weights such that \apsshort impacting read and write performance are ranked on the top followed by other \apsshort which impact data amplification, maintainability and accuracy. 

\sys reported \apsshort which were introduced by the third-party libraries used by the applications. The issue we raised on github and google forums, started the conversation on evaluating their design decisions.
