# Supplementary material for: SQLCheck: Automated Detection and Diagnosis of SQL Anti-Patterns
Source: arXiv:2004.10232 source file (2020-04-21)
Supplement: Supplementary file 5 [file performance-evaluation.tex]

\section{Performance Impact}
In this we list more performance impact metrics of \apshort in addition to the once mentioned in \cref{evaluation::ranking-repair}. 

\begin{figure*}[t]
\subfloat[][Index Overuse:\\ Delete]{
\includegraphics[width=0.13\textwidth]{"charts/globaleaks/INDEX-OVER-USE/altair-INDEX OVER USE-Delete-barchart-errorbars".pdf}
\label{fig:index-overuse-delete}
}
\qquad
\subfloat[][Index Overuse:\\ Insert]{
\includegraphics[width=0.13\textwidth]{"charts/globaleaks/INDEX-OVER-USE/altair-INDEX OVER USE-Delete-barchart-errorbars".pdf}
\label{fig:index-overuse-delete}
}
\qquad
\subfloat[][No Primary Key:\\ Select]{
\includegraphics[width=0.13\textwidth]{"charts/globaleaks/NO-PRIMARY-KEY/altair-NO PRIMARY KEY-Select, Join-barchart-errorbars".pdf}
\label{fig:index-overuse-delete}
}
\qquad
\subfloat[][Column Wildcard Usage: Select]{
\centering
\includegraphics[width=0.13\textwidth]{"charts/globaleaks/SELECT-STAR/altair-SELECT STAR-Select-barchart-errorbars".pdf}
\label{fig:select-star}
}
\qquad
\caption{
\textbf{Ranking and Repair of \apshort:} Performance impact of \apshort on
different types of \sql statements.}
\end{figure*}

\begin{figure}[t]
\centering
\subfloat[Task \#1]{
\includegraphics[width=0.13\textwidth]{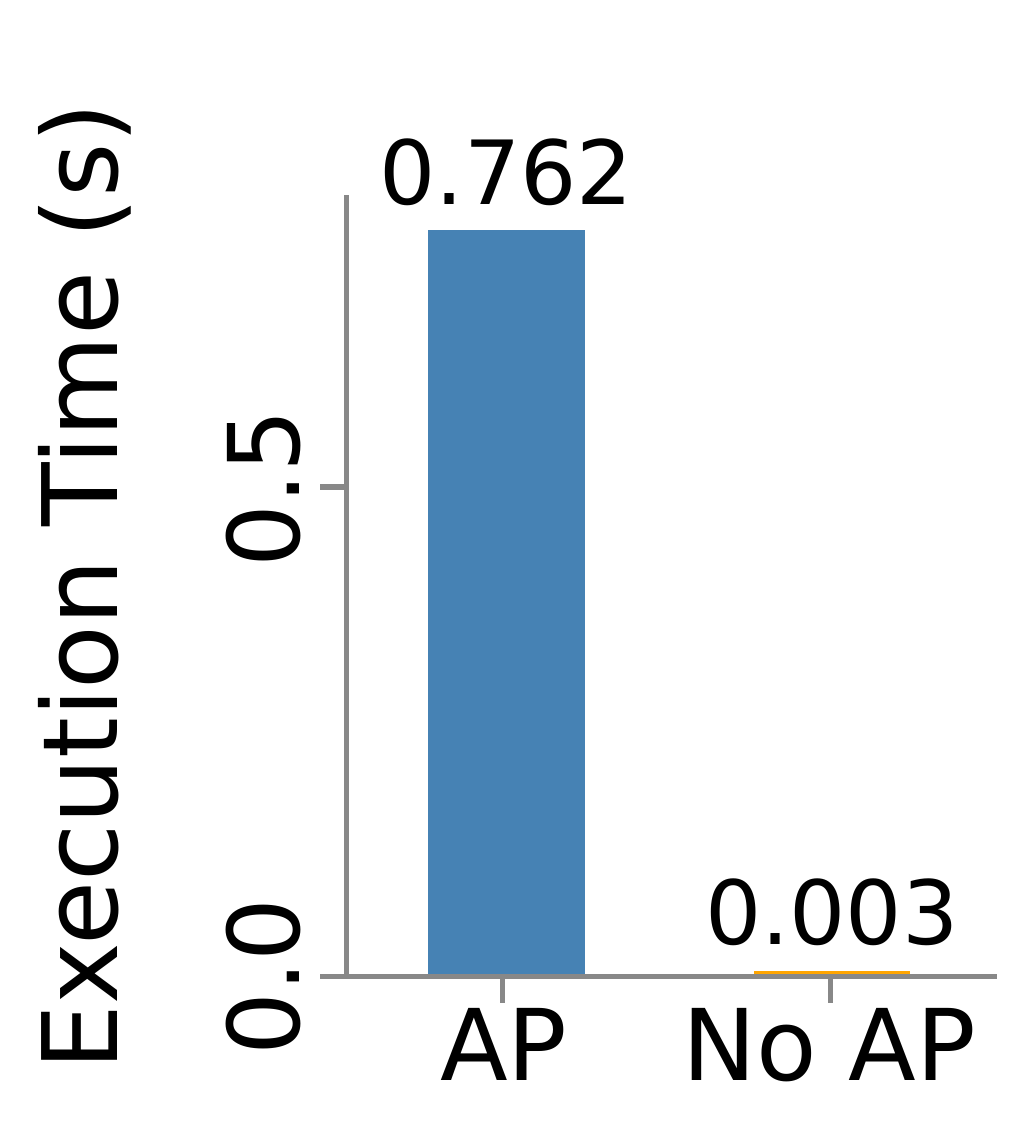}
\label{fig:mva-delete}
}
% \qquad
\subfloat[Task \#2]{
\includegraphics[width=0.13\textwidth]{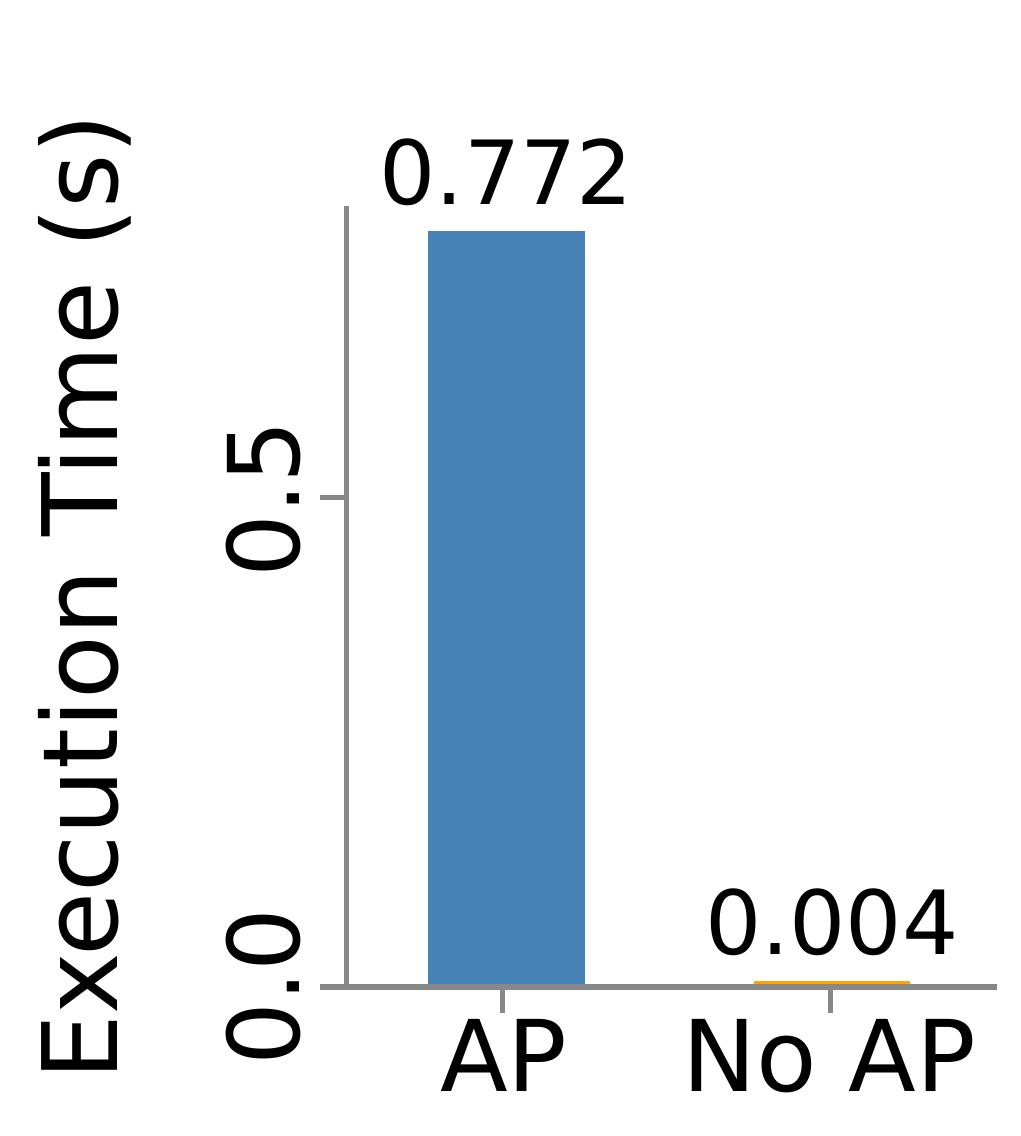}
\label{fig:mva-insert}
}
% \\
\subfloat[Task \#3]{
\includegraphics[width=0.13\textwidth]{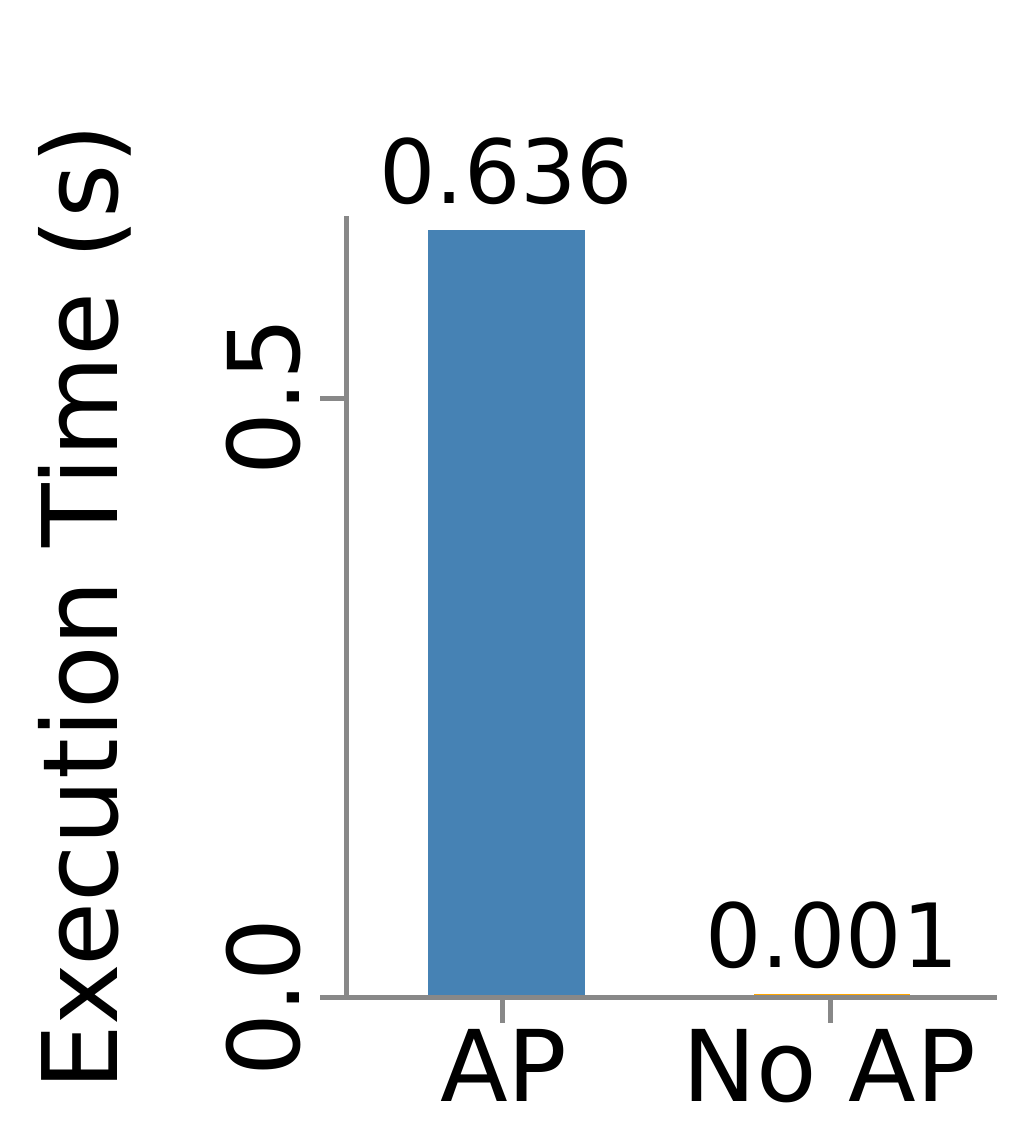}
\label{fig:mva-select}
}
%\\
% \qquad
%\subfloat[Task \#4]{
%\includegraphics[width=0.13\textwidth]{"charts/globaleaks/MULTIVALUED-ATTRIBUTES/altair-MULTIVALUED
%% ATTRIBUTES-JOIN-barchart-errorbars".pdf}
%\label{fig:mva-join}
%}
\caption{
\textbf{Multi-Valued Attribute \apshort:} Performance impact of the 
multi-valued attribute \apshort on the above-mentioned tasks.
}
\label{fig:mva-box}
\end{figure}
% \cref{fig:mva-box} shows the impact MVA anti-pattern has on performance.
